# Supplementary material for: Enhanced Superconductivity in Proximity to Peaks in Densities of States
Source: arXiv:2512.11451 ancillary file (2026-03-24)
Supplement: Supplementary file 1 [file Supplemental_material_for_Enhanced_Superconductivity_in_Proximity_to_Peaks_in_Densities_of_States.pdf]

# Supplemental material for Enhanced Superconductivity in Proximity to Peaks in Densities of States

Joshua Althüser,* Ilya M. Eremin,† and Götz S. Uhrig‡
*TU Dortmund University, Otto-Hahn Straße 4, 44227 Dortmund, Germany and*
*Theoretische Physik III, Ruhr-Universität Bochum, 44801 Bochum, Germany*
(Dated: December 12, 2025)

This supplement consists of multiple sections. In Section I, we derive the effective electron-electron coupling employed in the main text. In Section II, we briefly discuss the renormalization of the chemical potential $\mu(T)$. In Section III, we show the effect of the Debye frequency $\omega_{\mathrm{D}}$ on the critical temperature $T_c$ and on the specific heat $C_V$. In Section IV, we discuss the effect of the Fermi level $E_{\mathrm{F}}$ on the same thermodynamic quantities. In Section V, we perform the same analysis as in the main text except that we additionally include a constant repulsive pseudopotential following the Anderson-Morel description [1]. In Section VI, we discuss some example quasiparticle densities of states.

The Hamiltonian of the system reads

$$\begin{aligned}\mathcal{H} &= \sum_{\boldsymbol{k}\sigma}(\varepsilon_{\boldsymbol{k}} - \mu)\hat{c}^\dagger_{\boldsymbol{k},\sigma}\hat{c}_{\boldsymbol{k},\sigma} \\ &- \frac{1}{N}\sum_{\boldsymbol{k}\boldsymbol{k}'\sigma} g(\boldsymbol{k},\boldsymbol{k}')\hat{c}^\dagger_{\boldsymbol{k},\sigma}\hat{c}^\dagger_{-\boldsymbol{k},-\sigma}\hat{c}_{-\boldsymbol{k}',-\sigma}\hat{c}_{\boldsymbol{k}',\sigma},\end{aligned} \tag{1}$$

where $\hat{c}^{(\dagger)}_{\boldsymbol{k},\sigma}$ annihilate (create) an electron with momentum $\boldsymbol{k}$ and spin $\sigma$, $\mu$ is the chemical potential, $\varepsilon_{\boldsymbol{k}}$ is the single-particle dispersion, and $N$ the number of lattice sites. We choose the hopping constant such that $\varepsilon \in [-W, W]$ with $2W$ being the full band width. The chemical potential $\mu(T)$ is computed self-consistently such that the filling is kept constant. We initialize the system with the Fermi energy $E_{\mathrm{F}}$ of the would-be normal state at $T = 0$. The effective interaction can be expressed in terms of the single-particle energies

$$g(\varepsilon, \varepsilon') = \frac{g}{2\tilde{\rho}}\Theta(\omega_{\mathrm{D}} - |\varepsilon - \varepsilon'|). \tag{2}$$

We define the dimensionless coupling strength $g$ and the average DOS close to the Fermi edge

$$\tilde{\rho} := \frac{1}{2\omega_{\mathrm{D}}}\int_{E_{\mathrm{F}}-\omega_{\mathrm{D}}}^{E_{\mathrm{F}}+\omega_{\mathrm{D}}} \mathrm{d}\varepsilon \rho(\varepsilon). \tag{3}$$

We choose the DOS of a bcc lattice with nearest-neighbor hopping given by [2]

$$\rho(\varepsilon) = -\frac{4}{\pi^3}\,\mathrm{Im}\left[z\left(K\left(\frac{1}{2} - \frac{1}{2}\sqrt{1 - z^2}\right)\right)^2\right], \tag{4}$$

where $z := 1/[\varepsilon/W + \mathrm{i}0^+]$ and $K(x)$ is the complete elliptic integral of the first kind. This DOS carries most of its weight in a logarithmic singularity at $\varepsilon = \varepsilon_{\mathrm{peak}} = 0$. We provide a plot of $\rho$ in the main text in Fig. 1(a).

We study the critical temperature $T_c$ and the heat capacity $C_V$, which are rendered accessible by standard mean-field decoupling of the interaction term. We obtain the self-consistency equation

$$\Delta(\varepsilon) = \frac{g}{\tilde{\rho}}\int \mathrm{d}\varepsilon' \rho(\varepsilon')\Theta(\omega_{\mathrm{D}} - |\varepsilon - \varepsilon'|)\frac{\Delta(\varepsilon')}{2E(\varepsilon')} \tag{5}$$

with the quasiparticle dispersion $E(\varepsilon) = \sqrt{(\varepsilon - E_{\mathrm{F}})^2 + \Delta^2(\varepsilon)}$. We solve this problem numerically using an energy mesh with 10000 equidistant points. The analysis of collective excitations is performed using the iterated equations of motion approach [3]. Unless stated otherwise, we set $\omega_{\mathrm{D}} = 0.04W$ and $E_{\mathrm{F}} = -0.5W$.

## I. DERIVATION OF THE EFFECTIVE ELECTRON-ELECTRON INTERACTION

Here, we briefly derive the effective electron-electron interaction, following the original derivation in Ref. [4]. We begin with a Hamiltonian including one phonon branch and the electron-phonon coupling

$$\begin{aligned}\mathcal{H} &= \sum_{\boldsymbol{k}}\sum_{\sigma}\varepsilon_{\boldsymbol{k}}\hat{c}^\dagger_{\boldsymbol{k},\sigma}\hat{c}_{\boldsymbol{k},\sigma} + \sum_{\boldsymbol{q}}\omega_{\boldsymbol{q}}\hat{b}^\dagger_{\boldsymbol{q}}\hat{b}_{\boldsymbol{q}} \\ &+ \sum_{\boldsymbol{k}\boldsymbol{q}}\sum_{\sigma}\left(M_{\boldsymbol{k},\boldsymbol{q}}\hat{b}^\dagger_{-\boldsymbol{q}}\hat{c}^\dagger_{\boldsymbol{k}+\boldsymbol{q},\sigma}\hat{c}_{\boldsymbol{k},\sigma} + \mathrm{H.\,c.}\right) \\ &+ \sum_{\boldsymbol{k}\boldsymbol{k}'\boldsymbol{q}}\sum_{\sigma\sigma'}V^{\mathrm{eff}}_{\boldsymbol{k},\boldsymbol{k}',\boldsymbol{q}}\hat{c}^\dagger_{\boldsymbol{k}+\boldsymbol{q},\sigma}\hat{c}^\dagger_{\boldsymbol{k}'-\boldsymbol{q},\sigma'}\hat{c}_{\boldsymbol{k}',\sigma'}\hat{c}_{\boldsymbol{k},\sigma}\end{aligned} \tag{6}$$

Here, $\hat{b}^{(\dagger)}_{\boldsymbol{q}}$ annihilates (creates) a phonon with momentum $\boldsymbol{q}$. The phonon dispersion is $\omega_{\boldsymbol{q}}$, and the electron-phonon coupling is $M_{\boldsymbol{k},\boldsymbol{q}}$. Initially, $M_{\boldsymbol{k},\boldsymbol{q}} \equiv M_{\boldsymbol{q}}$ is independent of the electron's momentum, but it will acquire such a dependence during the calculations. Similarly, the effective electron-electron interaction $V^{\mathrm{eff}}_{\boldsymbol{k},\boldsymbol{k}',\boldsymbol{q}}$ initially vanishes identically, but becomes finite as the subsystems are decoupled. We assume inversion symmetry $\varepsilon_{\boldsymbol{k}} = \varepsilon_{-\boldsymbol{k}}$ and $\omega_{\boldsymbol{q}} = \omega_{-\boldsymbol{q}}$. The normalization constant $1/\sqrt{N}$ is absorbed in $M_{\boldsymbol{k},\boldsymbol{q}}$.

* joshua.althueser@tu-dortmund.de
† ilya.eremin@ruhr-uni-bochum.de
‡ goetz.uhrig@tu-dortmund.de

We decouple the electronic and phononic degrees of freedom by employing a continuous unitary transformation (CUT) [4–6]. To this end, one needs to solve the flow equation

$$\partial_\ell \mathcal{H}(\ell) = [\eta(\ell), \mathcal{H}(\ell)]. \tag{7}$$

The flow is initialized at $\ell = 0$ with Eq. (6). For $\ell \to \infty$, we obtain the effective, decoupled Hamiltonian.

The decoupling is achieved by employing the generator [4]

$$\begin{aligned}\eta(\ell) = &\sum_{\boldsymbol{kq}}\sum_{\sigma} \mathrm{sgn}[\alpha(\boldsymbol{k},\boldsymbol{q})] M_{\boldsymbol{k},\boldsymbol{q}}(\ell) \hat{b}^\dagger_{-\boldsymbol{q}} \hat{c}^\dagger_{\boldsymbol{k}+\boldsymbol{q},\sigma}\hat{c}_{\boldsymbol{k},\sigma} \\ &+ \sum_{\boldsymbol{kq}}\sum_{\sigma} \mathrm{sgn}[\beta(\boldsymbol{k},\boldsymbol{q})] M^*_{\boldsymbol{k}+\boldsymbol{q},-\boldsymbol{q}}(\ell) \hat{b}_{\boldsymbol{q}} \hat{c}^\dagger_{\boldsymbol{k}+\boldsymbol{q},\sigma}\hat{c}_{\boldsymbol{k},\sigma} \end{aligned} \tag{8}$$

with the abbreviations

$$\alpha(\boldsymbol{k},\boldsymbol{q}) = \varepsilon_{\boldsymbol{k}+\boldsymbol{q}}(\ell) - \varepsilon_{\boldsymbol{k}}(\ell) + \omega_{\boldsymbol{q}}(\ell) \tag{9a}$$

$$\beta(\boldsymbol{k},\boldsymbol{q}) = \varepsilon_{\boldsymbol{k}+\boldsymbol{q}}(\ell) - \varepsilon_{\boldsymbol{k}}(\ell) - \omega_{\boldsymbol{q}}(\ell) = -\alpha(\boldsymbol{k}+\boldsymbol{q},-\boldsymbol{q}). \tag{9b}$$

This generator does not extend the virtual processes beyond $|\varepsilon_{\boldsymbol{k}+\boldsymbol{q}} - \varepsilon_{\boldsymbol{k}}| \leq \omega_{\boldsymbol{q}}$ [7–9].

We are only interested in the effective electron-electron interaction up to $\mathcal{O}(M^2)$ and drop higher-order contributions. This procedure yields the flow equation for the electron-phonon coupling

$$\partial_\ell M_{\boldsymbol{k},\boldsymbol{q}}(\ell) = -|\alpha(\boldsymbol{k},\boldsymbol{q})| M_{\boldsymbol{k},\boldsymbol{q}}(\ell) \tag{10a}$$

$$\Rightarrow M_{\boldsymbol{k},\boldsymbol{q}}(\ell) = M_{\boldsymbol{q}} e^{-|\alpha(\boldsymbol{k},\boldsymbol{q})|\ell} + \mathcal{O}(M^3). \tag{10b}$$

The solution is accurate in $\mathcal{O}(M^2)$ because the electronic dispersion $\varepsilon_{\boldsymbol{k}}$ becomes $\ell$-dependent only in $\mathcal{O}(M^2)$. Notably, the electron-phonon coupling is eliminated for $\ell \to \infty$, unless $\alpha(\boldsymbol{k},\boldsymbol{q}) = 0$. However, these specific points in a six-dimensional parameter space, spanned by $\boldsymbol{k}$ and $\boldsymbol{q}$, form a null set and may be ignored.

Using Eq. (10b), the effective electron-electron interaction is expressed as

$$\partial_\ell V^{\mathrm{eff}}_{\boldsymbol{k},\boldsymbol{k}',\boldsymbol{q}}(\ell) = [\mathrm{sgn}[\beta(\boldsymbol{k}',-\boldsymbol{q})] - \mathrm{sgn}[\alpha(\boldsymbol{k},\boldsymbol{q})]]\, |M_{\boldsymbol{q}}|^2 \exp\left[-(|\alpha(\boldsymbol{k},\boldsymbol{q})| + |\alpha(\boldsymbol{k}'-\boldsymbol{q},\boldsymbol{q})|)\ell\right] \tag{11a}$$

$$\Rightarrow V^{\mathrm{eff}}_{\boldsymbol{k},\boldsymbol{k}',\boldsymbol{q}}(\infty) = |M_{\boldsymbol{q}}|^2 \left[\frac{\mathrm{sgn}[\alpha(\boldsymbol{k},\boldsymbol{q})] - \mathrm{sgn}[\beta(\boldsymbol{k}',-\boldsymbol{q})]}{|\alpha(\boldsymbol{k},\boldsymbol{q})| + |\beta(\boldsymbol{k}',-\boldsymbol{q})|}\right]. \tag{11b}$$

As before, this result is accurate in $\mathcal{O}(M^2)$. Notably, this perturbative expansion is the only approximation made to arrive at this result. As we chiefly care about superconductivity and not about renormalizations of the single-particle dispersion, we extract the BCS channel

$$\begin{aligned} g(\boldsymbol{k},\boldsymbol{k}') &:= V^{\mathrm{eff}}_{\boldsymbol{k},\boldsymbol{k}',\boldsymbol{q}} \\ &= -\frac{|M_{\boldsymbol{k}'-\boldsymbol{k}}|^2}{\omega_{\boldsymbol{k}'-\boldsymbol{k}}} \Theta\left(\omega_{\boldsymbol{k}'-\boldsymbol{k}} - |\varepsilon_{\boldsymbol{k}} - \varepsilon'_{\boldsymbol{k}}|\right). \end{aligned} \tag{12}$$

Choosing $|M_{\boldsymbol{k}'-\boldsymbol{k}}|^2 = \mathrm{const}$ and $\omega_{\boldsymbol{k}'-\boldsymbol{k}} = \omega_{\mathrm{D}} = \mathrm{const}$ yields Eq. (2).

Note that this potential is always attractive and the interaction is cut off sharply if $|\varepsilon_{\boldsymbol{k}} - \varepsilon'_{\boldsymbol{k}}| > \omega_{\boldsymbol{k}'-\boldsymbol{k}}$. In general, this does not need to be the case as unitary transformations that achieve such a decoupling are not unique [4, 10]. For example, in his foundational work, Fröhlich provided a result that is only attractive for momenta close to the Fermi level [11]. Moreover, a result similar to ours was derived by Lenz and Wegner [5]. While their result is also always attractive, the interaction strength merely decreases as a power-law in $|\varepsilon_{\boldsymbol{k}} - \varepsilon_{\boldsymbol{k}'}|^{-2}$. These comparisons, also presented in Ref. [4], highlight the advantages of the calculations described here.

## II. THE CHEMICAL POTENTIAL

As mentioned above, we fix the filling $n$ to the filling of the would-be normal state with $\mu = E_{\mathrm{F}}$ at $T = 0$. That is

$$n = 2\int_{-W}^{E_{\mathrm{F}}} \mathrm{d}\varepsilon \rho(\varepsilon). \tag{13}$$

where 2 refers to the spin degeneracy. Demanding this filling to remain constant implicitly defines the chemical potential $\mu$ as a function of both $g$ and $T$.

Figure 1 shows plots of $\mu(T) - E_{\mathrm{F}}$ for various $g$. Note that this shift remains rather small in all considered cases. The dotted line is the chemical potential of the would-be normal state. The thick lines represent the first line shown with $g > g_{\mathrm{enh}}$. We used the same parameters as in the main text for panel (a). For panels (b) and (c), we additionally considered the repulsion introduced by Morel and Anderson, cf. Section V.

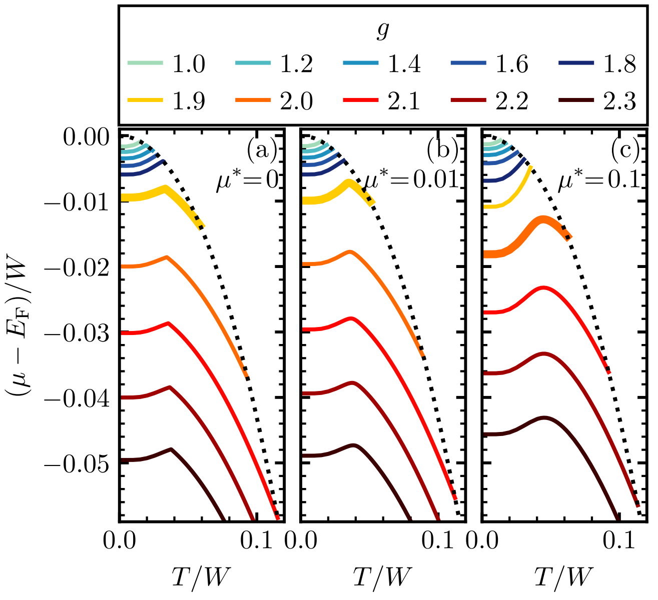


FIG. 1. Calculated chemical potential shift relative to $E_F$ as a function of the temperature $T$ for various interaction strengths $g$. The dotted line is the chemical potential of the would-be normal state. The individual panels (a–c) use different Anderson-Morel repulsions $\mu^*$. The thick line in each panel marks the first line with $g > g_{enh}$.

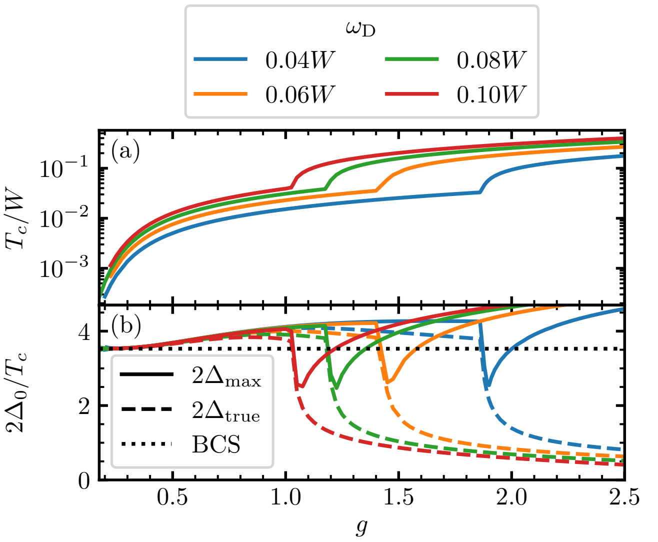


FIG. 2. (a) Calculated critical temperature $T_c$ as a function of the interaction strength $g$. The $y$-axis is scaled logarithmically. (b) Ratio of the maximum value of the order parameter $\Delta_{max}$ (solid lines) and energy gap of the quasiparticle dispersion $\Delta_{true}$ (dashed lines) at $T = 0$ to $T_c$ as a function of the interaction strength $g$. The black dotted line marks the BCS ratio ($\approx 3.528$) [12].

In any case, as expected, the $\mu$ of the superconducting system approaches the $\mu$ of the normal state system for $T \to T_c$. If $g < g_{enh}$, the chemical potential rises slightly as $T \to T_c$. For $g > g_{enh}$, $\mu(T)$ reaches a maximum and then rapidly decreases until reaching $T_c$.

The existence of such a maximum provides a more robust definition of $g_{enh}$: $g_{enh}$ is the first $g$, at which $\mu(T)$ exhibits a local maximum. This definition works even if the conventional and enhanced contributions overlap and is used throughout this supplement.

## III. EFFECT OF THE DEBYE FREQUENCY

We begin by studying the effect of varying $\omega_D$. In Fig. 2(a), we plot $T_c$ as a function of the interaction strength $g$. The blue curve is the same as in the main text with $\omega_D = 0.04W$. The three other curves correspond to different $\omega_D$. Notably, the same enhancement of $T_c$ exists for all depicted cases. The only difference is the threshold interaction $g_{enh}$ at which this phenomenon occurs. Generally, a larger Debye frequency, or equivalently, a smaller electronic bandwidth $2W$, causes the enhancement to set in at smaller values of $g$.

In Fig. 2(b), we plot the maximum of the order parameter $\Delta_{max}$ (solid lines) and the energy gap $\Delta_{true}$ (dashed lines) in units of $T_c$. The dotted line marks the BCS ratio $\approx 3.528$ [12]. We find the same behavior in all cases. In the weak-coupling regime, we recover the BCS prediction. For intermediate coupling, we observe that $\Delta_{true} < \Delta_{max}$, due to the shift of the minimum of the quasiparticle dispersion, cf. Ref. [13]. At $g = g_{enh}$, the ratios plummet and only $\Delta_{max}/T_c$ recovers. The analysis of this feature is the same as provided in the main text.

In Fig. 3, we plot the specific heat as a function of the temperature with (a) $\omega_D = 0.06W$ and (b) $\omega_D = 0.08W$. The solid lines mark $T < T_c$, while the dashed lines mark $T > T_c$. The grayscale lines represent $g < g_{enh}$, in which case we qualitatively find the BCS behavior. The colorful lines mark $g > g_{enh}$. Here, we initially observe the same feature as in the main text: the conventional contribution at $\Delta(E_F)$ vanishes before the enhanced contribution $\Delta(\varepsilon_{peak})$ does. This induces an additional discontinuity in $C_V$ before the system enters the normal phase. However, as $g$ increases further, the conventional and enhanced contributions overlap. Then, the aforementioned discontinuity smears out. This behavior is clearly noticeable for large $g$ in Fig. 3b.

## IV. EFFECT OF THE FERMI ENERGY

Next, we perform the same analysis as in the previous section but for the Fermi energy $E_F$. Figure 4(a) again depicts $T_c$ as a function of $g$. If $E_F$ is sufficiently far away from the logarithmic divergence of the DOS at $\varepsilon = \varepsilon_{peak} = 0$, we find the same behavior as described in the main text: The critical temperatures significantly increase upon passing the threshold $g_{enh}$. However, this enhancement weakens as the Fermi energy approaches 0.

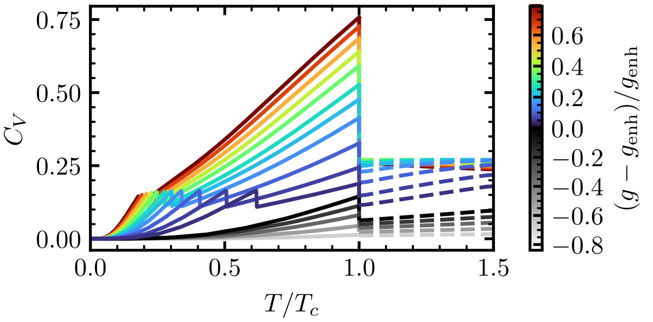


(a) $\omega_{\rm D} = 0.06W$, $g_{\rm enh} \approx 1.4$

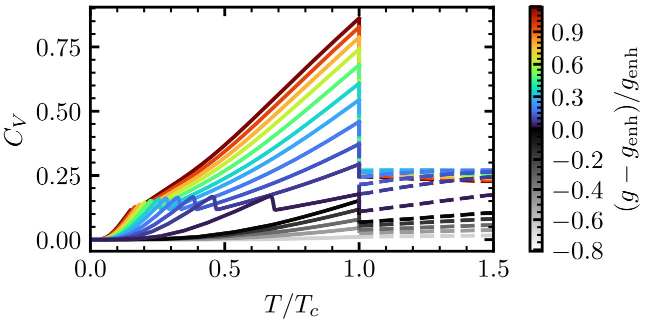


(b) $\omega_{\rm D} = 0.08W$, $g_{\rm enh} \approx 1.175$

FIG. 3. Calculated specific heat $C_V$ as a function of the temperature $T$. We used (a) $\omega_{\rm D} = 0.06W$ and (b) $\omega_{\rm D} = 0.08W$. The different colors indicate different coupling strengths $g$ as indicated by the colorbar. The solid lines indicate the superconducting state, while the dashed lines indicate the normal state. For $g < g_{\rm enh}$ (in grayscale), we observe renormalized BCS behavior. For $g > g_{\rm enh}$ (colored), we find qualitatively unexpected behavior due to the enhanced SC away from $E_{\rm F}$.

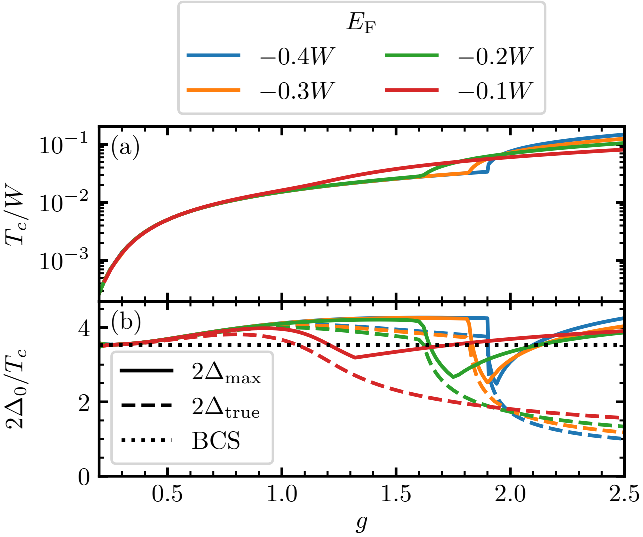


FIG. 4. Same as Fig. 2 except that $E_{\rm F}$ is varied.

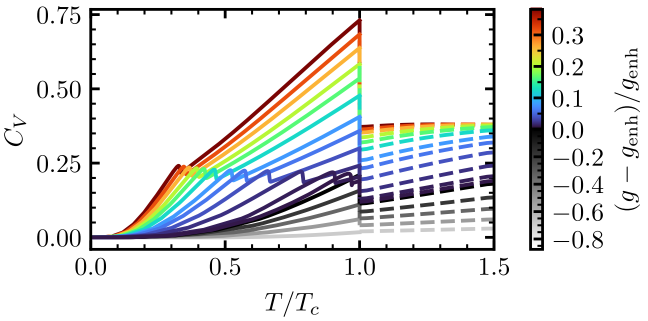


(a) $E_{\rm F} = -0.3W$, $g_{\rm enh} \approx 1.81$

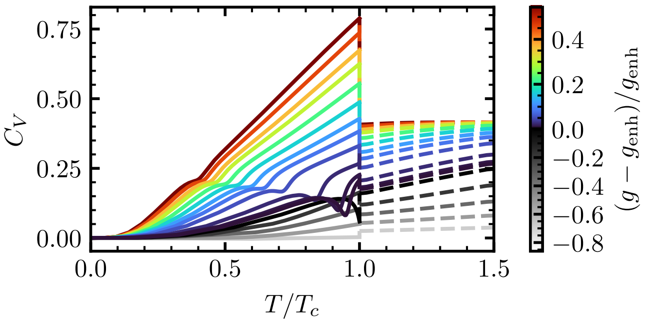


(b) $E_{\rm F} = -0.2W$, $g_{\rm enh} \approx 1.62$

FIG. 5. Same as Fig. 3 except that $E_{\rm F}$ is varied.

For $E_{\rm F} = -0.1W$, the enhancement is barely noticeable anymore. This behavior occurs because the contributions of $\Delta(E_{\rm F})$ and $\Delta(\varepsilon_{\rm peak})$ merge as $E_{\rm F} \to 0$. Thus, it becomes impossible to distinguish between an enhanced and a conventional contribution.

The ratios of the energy gap $2\Delta_{\rm true}$ and of the maximum of the order parameter $\Delta_{\rm max}$ to $T_c$ reflect the same behavior. If the Fermi energy is sufficiently far away from 0, the ratios plummet at $g = g_{\rm enh}$. As before, $2\Delta_{\rm true}/T_c$ remains at a low value as the energy gap is not affected by the order parameter far away from the Fermi edge. The value $E_{\rm F} = -0.1W$ presents an interesting marginal case. Here, the ratios never drop. Yet, there is a kink in $2\Delta_{\rm max}/T_c$, when $|\Delta(\varepsilon_{\rm peak})| > |\Delta(E_{\rm F})|$. As before, the energy gap itself remains unaffected. Hence, $2\Delta_{\rm true}/T_c$ remains smooth, but decreases substantially due to the increased critical temperature.

Next, we turn to the calculations of te specific heat $C_V$ plotted in Fig. 5. For Fig. 5a we set $E_{\rm F} = -0.3W$ and essentially find the same behavior as in the main text: For $g < g_{\rm enh}$, $C_V$ behaves in the BCS fashion, while for $g > g_{\rm enh}$, $C_V$ initially increases and then drops discontinuously. This discontinuity smears out for sufficiently large $g$ when the enhanced and conventional contributions to the order parameter overlap. This overlap occurs much faster for $E_{\rm F} = -0.2W$ in Fig. 5b. Moreover, the overlap is considerably larger, which is why the valley of low values of $C_V$ disappears almost entirely for large $g$.

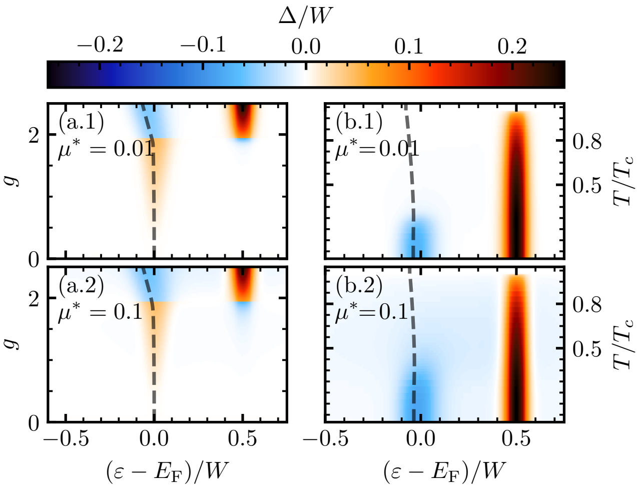


FIG. 6. (a) Calculated order parameter $\Delta$ at $T = 0$ as a function of the interaction strength $g$ and the single-particle energy $\varepsilon$. The sign of $\Delta$ is chosen such that $\Delta(W) < 0$. The almost vertical dashed line marks the chemical potential $\mu$. (b) Order parameter $\Delta$ as a function of the temperature $T$ for $g = 2.2 > g_{\mathrm{enh}}$. The upper row (1) depicts the data for $\mu^* = 0.01$, while the lower row (2) depicts the data for $\mu^* = 0.1$. Note that the order parameter does not entirely vanish at the Fermi edge, but is severely reduced by higher temperatures. The enhanced contribution at the singularity of the DOS at $\varepsilon = \varepsilon_{\mathrm{peak}}$ remains the dominant contribution at larger $T$. At $T_c$, the system enters the normal phase. The order parameter exhibits no features beyond the $\varepsilon$-range depicted in the plots.

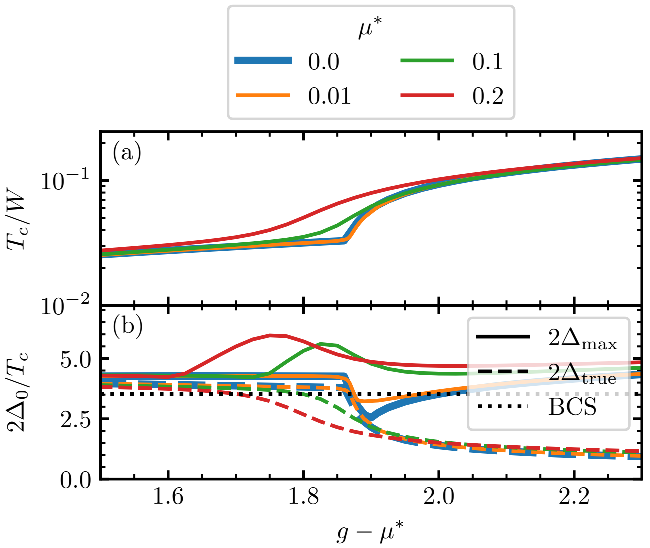


FIG. 7. Same as Fig. 2 except that we included the repulsive pseudopotential $\mu^*$. Additionally, we vary $g - \mu^*$ along the $x$-axis and restrict the plot to the values of $g$ near $g_{\mathrm{enh}}$. The lines for $\mu^* = 0$ (blue) and $\mu^* = 0.01$ (orange) are almost identical.

## V. EFFECT OF A REPULSIVE PSEUDOPOTENTIAL

In order to assess how additional interactions, such as Coulomb interactions, influence the scenario of enhanced superconductivity exposed in the main text, we turn to the theory of Morel and Anderson [1]. They stated that a screened Coulomb interaction's effect on the order parameter is effectively the same as a constant repulsive pseudopotential described by

$$\mathcal{H}_{\mathrm{AM}} = \frac{\mu^*}{2\tilde{\rho}} \frac{1}{N} \sum_{\boldsymbol{k}\boldsymbol{k}'\sigma} \hat{c}^\dagger_{\boldsymbol{k},\sigma} \hat{c}^\dagger_{-\boldsymbol{k},-\sigma} \hat{c}_{-\boldsymbol{k}',-\sigma} \hat{c}_{\boldsymbol{k}',\sigma}. \tag{14}$$

Typical values of $\mu^*$ are in the order of 0.1 [1]. In their derivation, Morel and Anderson considered a parabolic electron dispersion relation, which is well justified for good metals. Even though this does not apply to our model, the effective Anderson-Morel potential allows us to estimate the influence of further interactions.

We begin by analyzing the order parameter. In Fig. 6(a), we plot $\Delta$ as a function of $g$ and $\varepsilon$. The upper row (1) depicts the results for $\mu^* = 0.01$, while the bottom row depicts the results for $\mu^* = 0.1$. In both cases, we use the U(1) phase symmetry of the model to fix the sign of the order parameter such that $\Delta(W) < 0$. The expected behavior of an averaged repulsive interaction on superconductivity is to extend $\Delta$ over all momenta, here all energies, and to induce a sign change [1, 13–17]. That is, if the main contribution is positive, then the order parameter is negative far from it. The condition $\Delta(W) < 0$ allows us to decide whether $\Delta(\varepsilon_{\mathrm{peak}})$ or $\Delta(E_{\mathrm{F}})$ is the dominant contribution: the dominant one will be positive in the chosen gauge. The enhanced contribution $\Delta(\varepsilon_{\mathrm{peak}})$ becomes dominant around $g \approx g_{\mathrm{enh}}$.

In Fig. 6(b), we study the order parameter as a function of $T$ for $g = 2.2 > g_{\mathrm{enh}}$. The upper panel with $\mu^* = 0.01$ is similar to the case presented in the main text, although the conventional and enhanced contributions have a different sign. The conventional contribution at $\varepsilon \approx E_{\mathrm{F}}$ almost entirely disappears at much lower temperatures than the enhanced contribution at $\varepsilon \approx \varepsilon_{\mathrm{peak}}$. Note that $\Delta(E_{\mathrm{F}})$ never completely vanishes for $T < T_c$. That means that the system is never completely gapless. The lower panel with $\mu^* = 0.1$ essentially displays the same behavior. The only notable difference is that the magnitude of the order parameter far away from the main contributions is larger due to the larger value of $\mu^*$.

Next, we study the evolution of the critical temperature $T_c$ in Fig. 7. As before, the upper panel (a) depicts $T_c$, while the lower panel (b) displays the ratios $2\Delta_{\mathrm{max}}/T_c$ and $2\Delta_{\mathrm{true}}/T_c$. For reference, we also plot the data of the main text with $\mu^* = 0$ (blue lines). Importantly, the data for $\mu^* = 0$ and $\mu^* = 0.01$ (orange lines) almost match indicating that the limit $\mu^* \to 0$ is captured by $\mu^* = 0$. For larger $\mu^*$ (green and red lines), there are a few qualitative changes. The critical temperature does not increase as abruptly upon reaching $g_{\mathrm{enh}}$. Nonetheless, an enhancement of $T_c$ persists; it merely occurs more smoothly as a function of $g$. The

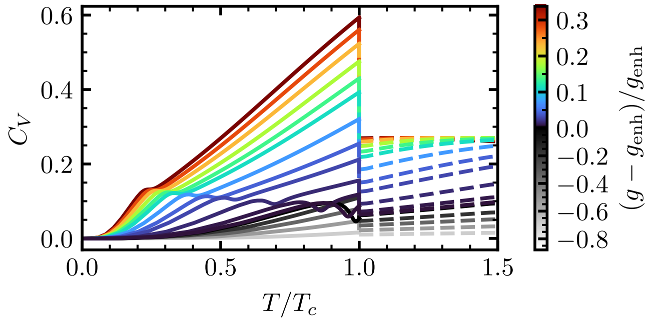


(a) $\mu^* = 0.01$, $g_{\mathrm{enh}} \approx 1.876$

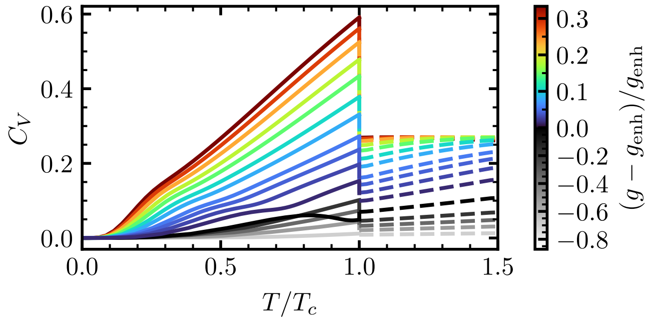


(b) $\mu^* = 0.1$, $g_{\mathrm{enh}} \approx 1.95$

FIG. 8. Same as Fig. 3 except that we included the repulsive effective potential $\mu^*$. We fixed $\omega_{\mathrm{D}} = 0.04W$ and set (a) $\mu^* = 0.01$ and (b) $\mu^* = 0.1$.

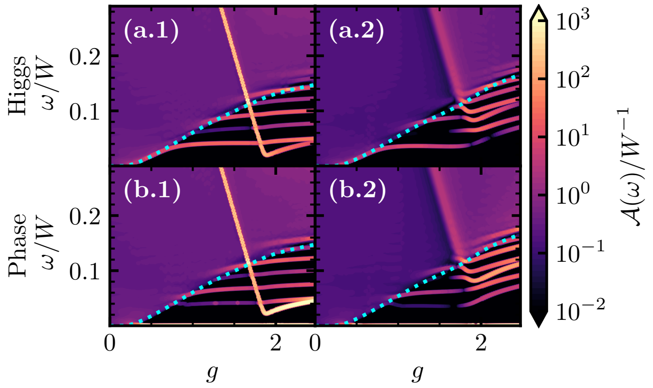


FIG. 9. Calculated zero temperature spectral functions (a) $\mathcal{A}_{\mathrm{Higgs}}(\omega)$ and (b) $\mathcal{A}_{\mathrm{Phase}}(\omega)$, represented by the color scale. The energy varies along the $y$-axis, and the interaction strength $g$ along the $x$-axis. The cyan dotted line marks the lower edge of the quasiparticle continuum at $2\Delta_{\mathrm{true}}$. The left panels (1) depict the data for $\mu^* = 0.01$, while the right panels depict the data for $\mu^* = 0.1$. The secondary modes found in Ref. [13] are clearly visible. Additionally, another mode rapidly decreases in energy. Within the continuum, the mode is less dominant than in the main text and does not soften completely. The artificial broadening is done as in Fig. 4 of the main text.

larger $\mu^*$, the smoother $T_c$ behaves.

The ratio $2\Delta_{\mathrm{max}}/T_c$ drops for $\mu^* = 0$ and $\mu^* = 0.01$ at $g \gtrsim g_{\mathrm{enh}}$. However, it rises for $\mu^* = 0.1$ and $\mu^* = 0.2$, even if $g$ is slightly smaller than $g_{\mathrm{enh}}$. In this region, $|\Delta(\varepsilon_{\mathrm{peak}})| > |\Delta(E_{\mathrm{F}})|$. Yet, the previously introduced condition $\Delta(W) < 0$ for the gauge entails $\Delta(E_{\mathrm{F}}) > 0$ and $\Delta(\varepsilon_{\mathrm{peak}}) < 0$. Thus, the conventional contribution at $\varepsilon \approx E_{\mathrm{F}}$ is still the dominant one. As $T_c$ increases more quickly upon reaching $g_{\mathrm{enh}}$, the ratio decreases again.

The ratio $2\Delta_{\mathrm{true}}/T_c$ behaves qualitatively the same in all considered cases. It decreases significantly for $g \gtrsim g_{\mathrm{enh}}$, though the decrease is slower the larger $\mu^*$ is because $T_c$ rises more slowly.

For the static thermodynamic quantities, we turn to the specific heat $C_V$. Figure 8a shows $C_V$ as a function of $T$ for various $g$ and $\mu^* = 0.01$. As before, the grayscale symbolizes BCS behavior, while the colored lines mark the enhanced behavior. The lines are dashed for $T > T_c$, i.e., in the normal phase. For $g > g_{\mathrm{enh}}$, we still observe a hilltop in $C_V$, when the conventional contribution to the order parameter vanishes except for a small residual value. The discontinuity present for vanishing $\mu^*$ is smeared out for finite values of $\mu^*$. The same argument as above applies here for large $\omega_{\mathrm{D}}$. Because $\mu^*$ is a constant interaction across the entire energy range, it effectively connects the conventional and enhanced contributions such that the enhanced contribution still has some effect at $\varepsilon = E_{\mathrm{F}}$.

Figure 8b displays the data for $\mu^* = 0.1$. The hilltop in $C_V$ is even more smeared out than before, though it is still noticeable. However, for very large $g$, the heat capacity approaches an almost straight line.

Finally, we investigate the changes to the spectra of collective excitations induced by $\mu^*$. As in the main text we proceed by evaluating the two-particle response functions $\mathcal{G}_\alpha(\omega)$ with respect to the operators

$$\mathfrak{A}_{\mathrm{Higgs}} = \frac{1}{\sqrt{N}} \sum_{\boldsymbol{k}} \left( \hat{c}^\dagger_{\boldsymbol{k},\uparrow} \hat{c}^\dagger_{-\boldsymbol{k},\downarrow} + \hat{c}_{-\boldsymbol{k},\downarrow} \hat{c}_{\boldsymbol{k},\uparrow} \right) \tag{15a}$$

$$\mathfrak{A}_{\mathrm{Phase}} = \frac{\mathrm{i}}{\sqrt{N}} \sum_{\boldsymbol{k}} \left( \hat{c}^\dagger_{\boldsymbol{k},\uparrow} \hat{c}^\dagger_{-\boldsymbol{k},\downarrow} - \hat{c}_{-\boldsymbol{k},\downarrow} \hat{c}_{\boldsymbol{k},\uparrow} \right), \tag{15b}$$

which allows us to capture the amplitude and phase channels, respectively. The calculation is done using the iterated equations of motion approach [3].

Figure 9 depicts the spectral functions $\mathcal{A}_\alpha(\omega) := (1/\pi)\mathcal{G}_\alpha(\omega)$ with (a) $\alpha = $ Higgs and (b) $\alpha = $ Phase. For the left column (1), we set $\mu^* = 0.01$. The global phase mode remains gapless at $\omega = 0$ because no proper long-range Coulomb interaction is included. The spectrum of secondary excitations, which was already presented in Ref. [13], is largely unaffected by this small additional interaction.

The mode associated with the enhanced second SC order remains fairly sharp even within the quasiparticle continuum. However, it does not become completely soft for finite $\mu^*$. Instead, its energy reaches a minimum around $g \approx g_{\mathrm{enh}}$ and then rises again.

In the right column (2), we set $\mu^* = 0.1$. The sharp collective mode has gained some width but remains

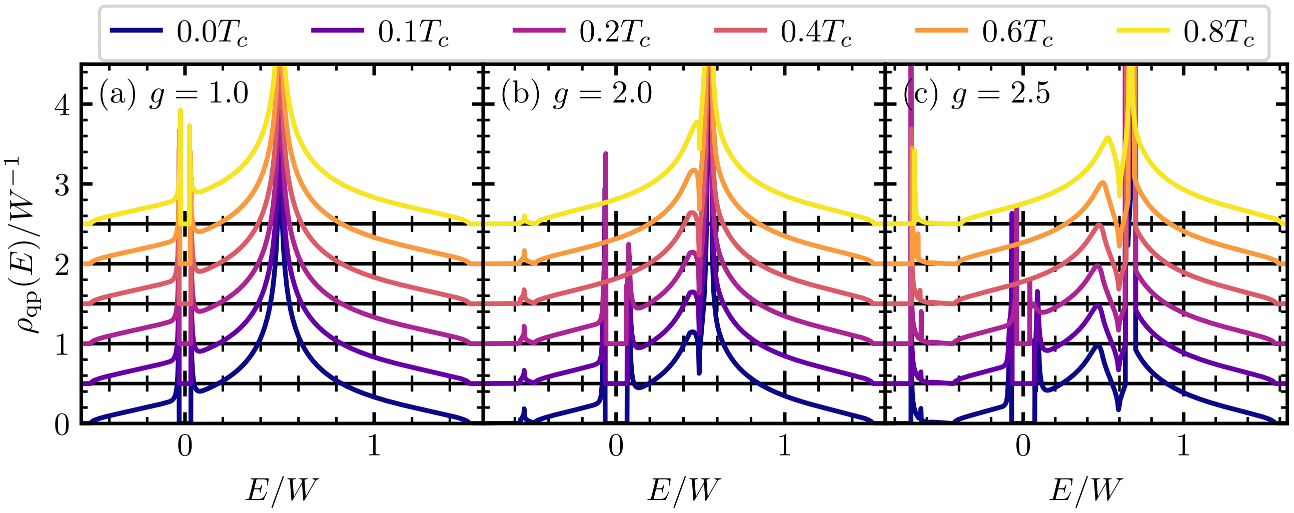


FIG. 10. Calculated quasiparticle density of states (16) for $\omega_{\mathrm{D}} = 0.04W$, $E_{\mathrm{F}} = -0.5W$, and $\mu^* = 0$. The individual panels (a–c) show the data for $g = 1, 2, 2.5$. Enhanced superconductivity occurs in panels (b) and (c). The different colors represent different temperatures in units of $T_c$ as given in the legend. The lines are shifted by 0.5 with respect to each other to improve visibility.

clearly discernible as a prominent resonance. It emerges from the continuum at $g \approx 1.8$, but remains at these energies, i.e, does not soften.

The results for finite Anderson-Morel parameters convey two messages. The first is that the scenario of two consecutive phase transitions, one to conventional order, one to enhanced superconductivity, is too idealized due to the mean-field treatment. The second message, however, is that features of the two kinds of orderings, conventional and enhanced, persist and should be detectable. They appear less abrupt and more smeared out in comparison to the results at $\mu^* = 0$.

## VI. THE QUASIPARTICLE DENSITY OF STATES

Finally, we discuss a few example quasiparticle densities of states (QP-DOS) defined by [18]

$$\rho_{\mathrm{qp}}(E) = \int_{-W}^{W} \mathrm{d}\varepsilon \rho(\varepsilon) \left[ u_\varepsilon^2 \delta(E - E(\varepsilon)) + v_\varepsilon^2 \delta(E + E(\varepsilon)) \right] \tag{16}$$

with the coherence factors

$$u_\varepsilon^2 = \frac{1}{2}\left(1 + \frac{\varepsilon - \mu}{E(\varepsilon)}\right), \qquad v_\varepsilon^2 = \frac{1}{2}\left(1 - \frac{\varepsilon - \mu}{E(\varepsilon)}\right). \tag{17}$$

This quantity can be readily measured experimentally, for instance, via tunnelling spectroscopy [19].

Figure 10 shows the QP-DOS for the parameters chosen in the main text $\omega_{\mathrm{D}} = 0.04W$, $E_{\mathrm{F}} = -0.5W$, and $\mu^* = 0$. In panel (a), $g = 1 < g_{\mathrm{enh}}$. Consequently, we find mostly BCS behavior, notwithstanding a slight asymmetry of the coherence peaks at $E = \pm\Delta_{\mathrm{true}}$. We attribute this asymmetry to the electronic DOS itself. In addition to the coherence peaks and the energy gap, we observe the underlying DOS of the bcc system at all temperatures.

In panel (b), $g = 2 > g_{\mathrm{enh}}$. Here, we again observe the energy gap and asymmetric coherence peaks at sufficiently low temperatures. As discussed in the main text, the gap vanishes at higher $T$ before the enhanced SC order disappears. Concurrently, the coherence peaks also disappear. However, we do not advocate for gapless SC, as other couplings, e.g., $\mu^*$, extend the order parameter over the entire parameter space.

Interestingly, the logarithmic singularity of the electronic DOS acquires additional structure as the enhanced order sets in around it. This manifests in a dip followed by a rapid increase in the QP-DOS. Simultaneously, the QP-DOS acquires substantial weight and another peak for $E < -\sqrt{(-W-\mu)^2 + \Delta^2(-W)}$. This weight appears around $E \approx -\sqrt{(\varepsilon_{\mathrm{peak}} - \mu)^2 + \Delta^2(\varepsilon_{\mathrm{peak}})}$. Thus, it is a mirrored effect of the structure at positive $E$ due to the presence of the enhanced order.

In panel (c), we increase $g = 2.5$. We observe the same features as in panel (b), but even more pronounced.

Figure 11 is analogous to Fig. 10, except that we set $E_{\mathrm{F}} = -0.2W$. For $g = 1 < g_{\mathrm{enh}}$ (a), we again observe mainly BCS behavior. The aforementioned asymmetry of the coherence peaks is more pronounced here, which we attribute to the steeper bare-electronic DOS.

For $g > g_{\mathrm{enh}}$ (b–c), we find a similar new structure around the previous logarithmic peak of the electronic DOS. Additionally, a mirrored structure, including corresponding peaks, manifests at $E \approx -\sqrt{(\varepsilon_{\mathrm{peak}} - \mu)^2 + \Delta^2(\varepsilon_{\mathrm{peak}})}$. This result clearly shows that this structure and the enhanced SC order are closely

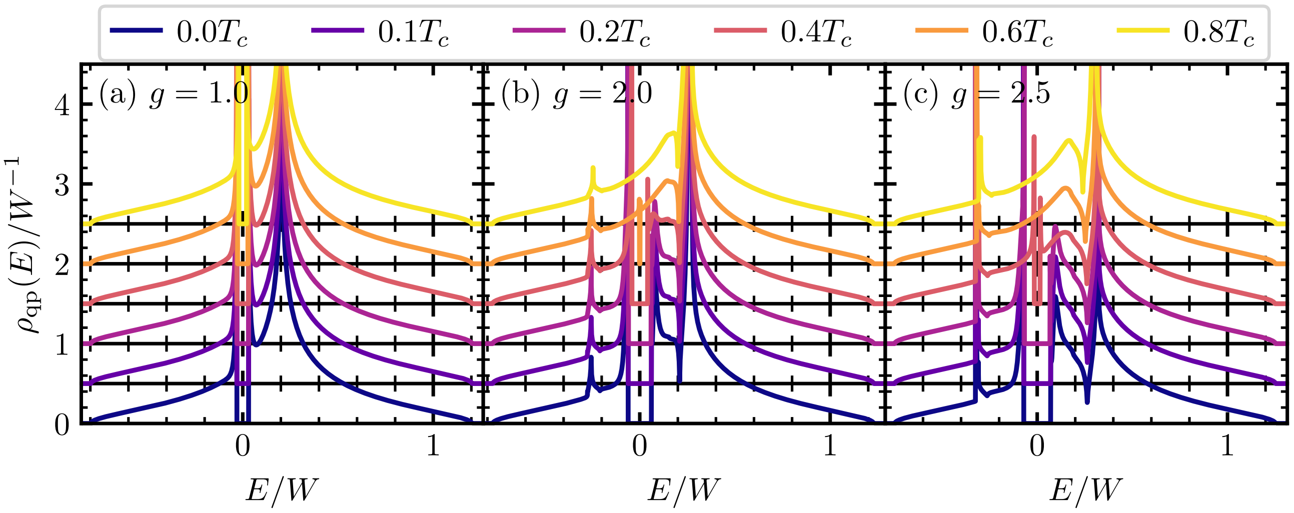


FIG. 11. Same as Fig. 10 except that $E_{\rm F} = -0.2W$.

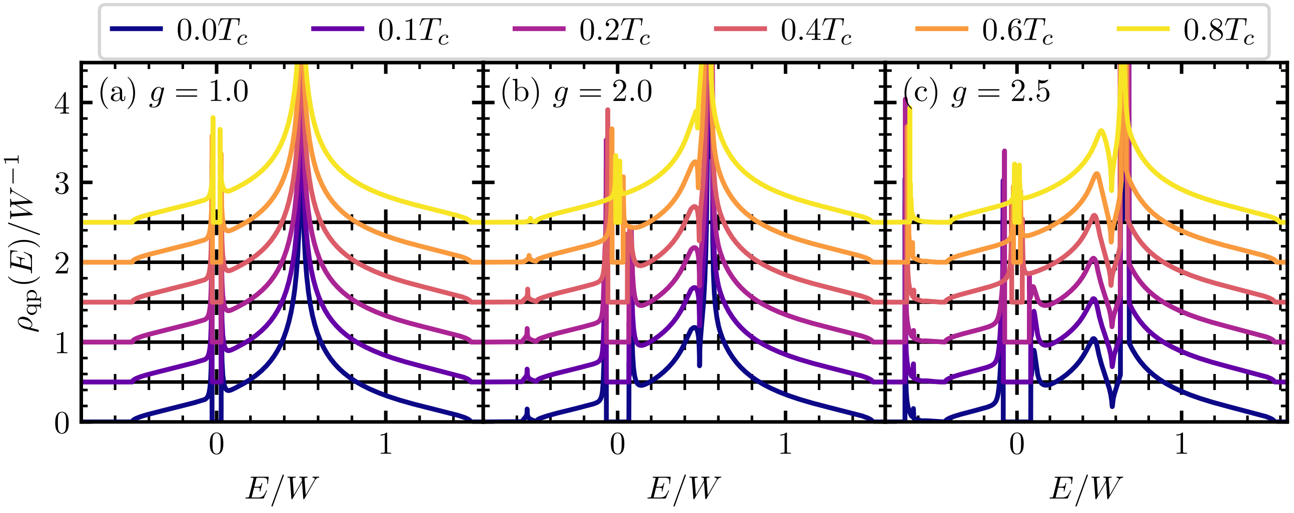


FIG. 12. Same as Fig. 10 except that $\mu^* = 0.1$.

linked.

Lastly, we show the QP-DOS for $\mu^* = 0.1$ in Fig. 12. As before, in panel (a) with $g = 1 < g_{\rm enh}$, we observe mainly BCS behavior, except for the aforementioned slight asymmetry of the coherence peaks.

The behavior in panels (b) and (c) is qualitatively the same as in Fig. 10, except that, as discussed before, the energy gap never truly vanishes for $T < T_c$. For clarification, we additionally provide a plot of the QP-DOS zoomed in around the energy gap in Fig. 13. In panel (a), we set $\mu^* = 0$ causing the energy gap to be exponentially suppressed, which appears as 0 in the numerics, for sufficiently large $T$. This does not happen in panel (b) with $\mu^* = 0.1$.

Other than that, we still observe the additional structure around the logarithmic singularity of the electronic DOS and at $E \approx -\sqrt{(\varepsilon_{\rm peak} - \mu)^2 + \Delta^2(\varepsilon_{\rm peak})}$.

In conclusion, these additional features are robust

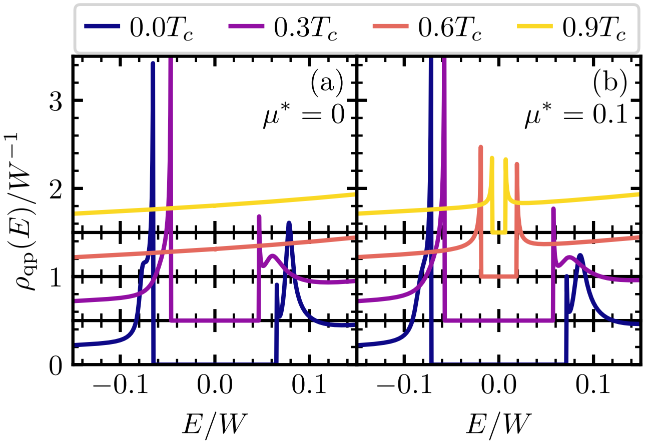


FIG. 13. QP-DOS for $g - \mu^* = 2$, $E_{\rm F} = -0.5W$ zoomed in around the energy gap. We set (a) $\mu^* = 0$ and (b) $\mu^* = 0.1$.

against the inclusion of additional, repulsive interactions. Thereby, we are able to predict an additional quantity that is readily accessible in experiments.


[1] P. Morel and P. W. Anderson, Calculation of the Superconducting State Parameters with Retarded Electron-Phonon Interaction, Physical Review **125**, 1263 (1962).

[2] G. S. Joyce, Exact evaluation of the body centred cubic lattice Green function, Journal of Physics C: Solid State Physics **4**, 1510 (1971).

[3] J. Althüser and G. S. Uhrig, Collective excitations in competing phases in two and three dimensions, Physical Review B **109**, 205153 (2024).

[4] H. Krull, N. A. Drescher, and G. S. Uhrig, Enhanced perturbative continuous unitary transformations, Physical Review B **86**, 125113 (2012).

[5] P. Lenz and F. Wegner, Flow equations for electron-phonon interactions, Nuclear Physics B **482**, 693 (1996).

[6] A. Mielke, Similarity renormalization of the electron-phonon coupling, Annalen der Physik **509**, 215 (1997).

[7] A. Mielke, Flow equations for band-matrices, The European Physical Journal B - Condensed Matter and Complex Systems **5**, 605 (1998).

[8] C. Knetter and G. Uhrig, The European Physical Journal B - Condensed Matter and Complex Systems **13**, 209 (2000).

[9] C. Heidbrink and G. Uhrig, Renormalization by continuous unitary transformations: One-dimensional spinless fermions, The European Physical Journal B - Condensed Matter and Complex Systems **30**, 443 (2002).

[10] S. Kehrein, *The Flow Equation Approach to Many-Particle Systems*, edited by G. Höhler, A. Fujimori, C. Varma, F. Steiner, J. Kühn, J. Trümper, P. Wölfle, and Müller, Springer Tracts in Modern Physics, Vol. 217 (Springer, 2006).

[11] H. Fröhlich, Interaction of electrons with lattice vibrations, Proceedings of the Royal Society of London. Series A. Mathematical and Physical Sciences **215**, 291 (1952).

[12] G. Czycholl, *Theoretische Festkörperphysik*, Springer-Lehrbuch (Springer, Berlin, Heidelberg, 2008).

[13] J. Althüser and G. S. Uhrig, Collective modes in superconductors including Coulomb repulsion, SciPost Physics **19**, 067 (2025).

[14] A. Mielke, Calculating critical temperatures of superconductivity from a renormalized Hamiltonian, Europhysics Letters **40**, 195 (1997).

[15] M. Sigrist, Introduction to Unconventional Superconductivity, AIP Conference Proceedings **789**, 165 (2005).

[16] M. Kostrzewa, R. Szczęśniak, J. K. Kalaga, and I. A. Wrona, Anomalously high value of Coulomb pseudopotential for the $h_5s_2$ superconductor, Scientific Reports **8**, 11957 (2018).

[17] M. Simonato, M. I. Katsnelson, and M. Rösner, Revised Tolmachev-Morel-Anderson pseudopotential for layered conventional superconductors with nonlocal Coulomb interaction, Physical Review B **108**, 064513 (2023).

[18] A. V. Chubukov, I. Eremin, and D. V. Efremov, Superconductivity versus bound-state formation in a two-band superconductor with small Fermi energy: Applications to Fe pnictides/chalcogenides and doped $SrTiO_3$, Physical Review B **93**, 174516 (2016).

[19] C. Wen, Z. Hou, A. Akbari, K. Chen, W. Hong, H. Yang, I. Eremin, Y. Li, and H.-H. Wen, Unprecedentedly large gap in $HgBa_2Ca_2Cu_3O_{8+\delta}$ with the highest $T_c$ at ambient pressure, npj Quantum Materials **10**, 20 (2025).
